# Supplementary material for: TreeSketchNet: From Sketch To 3D Tree Parameters Generation
Source: arXiv:2207.12297 source file (2022-10-27)
Supplement: Supplementary file 1 [file appendix.tex]

\section{Appendix: Render Tree parameters}\label{sec:appendix}
As mentioned in the section~\ref{sub:dataset_creation} our RT Blender add-on is based on the well-known Sapling Tree Gen. The parameters we used through RT add-on to reconstruct the 3D trees can be organized into five classes: geometry, branch radius, branch splitting, branch growth, and leaves. Although there are other classes, such as pruning, armature, and animation, we don't describe their parameters because we do not take into consideration such values for our trees and where there are mandatory we set them as a default values.  

\subsection{Geometry}\label{sub:geometry}
This class represents parameters that define the general tree geometry and its level of detail (LOD).
\begin{itemize}
    \item \textbf{Bevel Resolution}: controls the surface smoothing of the tree;
    \item \textbf{Handle Type}: represents the curve points type (we used the default value \textit{auto});
    \item \textbf{Shape}: sets the basic shape of the tree, by choosing among $9$, \eg conical, inverse conical, cylindrical, spherical \etc. There is a tenth value which activate the \textbf{customShape} parameter consisting of $4$ values, one for each tree level, trunk, branches of the first, second, and third level, as shown in Figure~\ref{fig:customShape}. Each value represents the length of component of each level;
    \begin{figure}[ht!]
        \centering
        \includegraphics[width=0.35\textwidth]{samples/\imageres/01_tree_levels.png}
        \caption{Length of tree components can be set with $4$ customShape values. Level 0 represents the trunk length, level 1 represents the first branches length, level 2 the second branches length, and the level 3 the fourth branches length}
        \label{fig:customShape}
    \end{figure}
    \item \textbf{Secondary Splits}: changes the style of secondary branches;
    \item \textbf{Branch Distribution}: defines the distribution of the branches by gathering them on the base or on the top of the trunk according to its value;
    \item \textbf{Branch Rings}: places branches around the trunk as a ring shape, providing also the number of rings (\eg Pine Tree);
    \item \textbf{Random Seed}: is useful to generate same type trees;
    \item \textbf{Scale} and \textbf{Scale Variation}: defines the base height of the tree.
\end{itemize}

\subsection{Branch Radius}\label{sub:branch_radius}
This class represents parameters useful to define the branches radius.
\begin{itemize}
    \item \textbf{Ratio}: is a branch thickness base value. 
    \item \textbf{Radius Scale} (scale0) and \textbf{Radius Scale Variation} (scaleV0): define the trunk radius scale and its variation range.
    \begin{equation}
        radius_{trunk} = length_{trunk} * ratio * (scale0 \pm scaleV0)
        \label{eq:radius_scale}
    \end{equation}
    where: $radius_{trunk}$ is the trunk radius, and $length_{trunk}$ is the trunk length;
    \item \textbf{Branch Radius Ratio} (ratioPower): defines the next level branches thickness value as follows: 
    \begin{equation}
        radius_{child}=radius_{parent}\left(\frac{length_{child}}{length_{parent}}\right)^{ratioPower}
        \label{eq:branch_radius}
    \end{equation}
    where: $radius_{child}$ is the previous branch radius, $radius_{parent}$ is the next branch radius, $length_{child}$ is the previous branch length, and $length_{parent}$ is the next branch length; 
    \item \textbf{Minimum Radius}: is the minimum radius value allowed for the thinnest branch;
    \item \textbf{Close Tip}: if selected, closes the tip of the branches;
    \item \textbf{Root Flare}: creates a conical shape at the base of the tree;
    \item \textbf{Taper}: contains a value for each level to define the branches tip thickness;
    \item \textbf{Tweak Radius}: contains a value for each level which is multiplied with Branch Radius Ratio (see \eqref{eq:branch_radius}) to keep major control on the branches thickness.
\end{itemize}

\subsection{Branch Splitting}\label{sub:branch_splitting}
This class contains the split of the branches parameters. Each level branches can be split, or cloned into other branches of the same level of the starting branch, as shown in Figure~\ref{fig:branch_splitting}.
\begin{figure}[ht!]
    \centering
    \includegraphics[width=0.45\textwidth]{samples/\imageres/02_segSplits_splitAngle.png}
    \caption{Branches splitting example.}
    \label{fig:branch_splitting}
\end{figure}
\begin{itemize}
    \item \textbf{Levels}: represents the number of branch levels, \eg with $levels=2$, a tree with trunk and first level branches will be generated;
    \item \textbf{Base Splits}: and Segment Split (described later) affect the trunk splitting;
    \item \textbf{Trunk Height}: indicates the trunk height percentage from which the branches are placed; 
    \item \textbf{Secondary Base Size}: decreases the base dimension for each level;
    \item \textbf{Split Height}: defines a height threshold below which there are no subdivisions in the tree;
    \item \textbf{Split Bias}: changes the splittings distribution by gathering them at the top or bottom of the tree; 
    \item \textbf{Branches}: number of branches for each level;
    \item \textbf{Segment Splits} (segSplits): number of splittings for each branch segment. With $segSplits = 0.0$ there is not splitting, with $segSplits = 1.0$ the branch is dichotomously  divided, with $segSplits = 2.0$ the branch is divided in three parts, and so on up $3$ as maximum value; 
    \item \textbf{Split Angle} and \textbf{Split Variation}: represent the angle amplitude and its variation;
    \item \textbf{Rotate Angle} and \textbf{Rotate Variation}: represent the direction grow angle and its variation, as shown in Figure~\ref{fig:branch_rationl} (left);
    \item \textbf{Branch Rotate}: represents the branch rotation angle for the branch rotation matrix, in which is defined also the rotation axis.
    \item \textbf{Rotation Last Angle}: is the last parent rotation which is summed with the current branch rotation to obtain the Branch Rotate parameter.
    \begin{figure}[ht!]
        \centering
        \includegraphics[width=0.195\textwidth]{samples/\imageres/03_rotate_rotateV.png}
        \includegraphics[width=0.195\textwidth]{samples/\imageres/04_curveRes.png}
        \caption{Branches rotation and curve resolution}
        \label{fig:branch_rationl}
    \end{figure}
    \item \textbf{Outward Attraction}: curve branches toward the external;
    \item \textbf{Branching Mode}: uniformly distributes the branches, allowing them to point toward external, starting from the branch center, or from the tree center, or randomly;  
    \item \textbf{Curve Resolution}: defines the sections number of each branch. Increasing such value more and more sinuous branches can be obtained (see Figure~\ref{fig:branch_rationl} (right)).
    \item \textbf{Sign}: defines sign of the angle obtained by summing the split angle and split angle variation.
\end{itemize}

\subsection{Branch Growth}\label{sub:branch_growth}
This class contains parameters to set the tree branches growth (see Figure~\ref{fig:branch_growth}). 
\begin{figure}[ht!]
    \centering
    \includegraphics[width=0.375\textwidth]{samples/\imageres/05_downAngle.png}
    \caption{Branches Growth}
    \label{fig:branch_growth}
\end{figure}
\begin{itemize}
    \item \textbf{Taper Crown}: decreases the trunk dimension and its respective subdivision;
    \item \textbf{Length} and \textbf{Length Variation}: determine respectively the branches length of each level and the variation range; 
    \item \textbf{Down Angle} (downAngle) and \textbf{Down Angle Variation}: pull back the branch, increasing the amplitude of the angle between it and the branch on which it grows (parent branch);
    \item \textbf{Curvature} and \textbf{Curvature Variation}: are useful to pull back the branches, curving them inwards;
    \item \textbf{Back Curvature}: curves the tips of the branches;
    \item \textbf{Vertical Attraction}: pull the branch towards the ground;
    \item \textbf{Use Old Down Angle Variation}: if selected, it uses the downAngle parameter of the previous branch (parent branch);
    \item \textbf{Use Parent Angle}: if selected, it rotates the branch to match the previous branch;
\end{itemize}

\subsection{Leaves}\label{sub:leaves}
This class contains parameters to set the foliage. The crown of the tree can be enabled or disabled as needed (see Figure~\ref{fig:foliage_parameters}).
\begin{figure}[ht!]
    \centering
    \includegraphics[width=0.35\textwidth]{samples/\imageres/06_leaf_horizontal.png}
    \caption{Foliage setting parameters}
    \label{fig:foliage_parameters}
\end{figure}
\begin{itemize}
    \item \textbf{Leaf Shape}: set the leaf shape, which can be rectangular, hexagonal, dupliface, or duplivert;
    \item \textbf{Leaves}: determines the leaves number for each branch;
    \item \textbf{Leaf Distribution}: indicates the leaves distribution type;
    \item \textbf{Leaf Down Angle} and \textbf{Leaf Down Angle Variation}: pull back the leaves, increasing the amplitude of the angle between it and the branch on which it grows (parent branch);
    \item \textbf{Leaf Rotation} and \textbf{Leaf Rotation Variation}: are the leaves direction grow angle and its variation; 
    \item \textbf{Leaf Scale} and \textbf{Leaf Scale Variation}: determine the leaves scale and its variation range;
    \item \textbf{Leaf Scale X}: scales the leaves along the X axis;
    \item \textbf{Leaf Scale Taper}: scales the leaves towards the tip or base of the branch on which they grow;
    \item \textbf{Horizontal Leaves}: if enabled, the leaves are turned upwards;
    \item \textbf{Leaf Angle}: pull the leaves towards the ground.
\end{itemize}
